# Supplementary material for: Multivariate Species Sampling Models
Source: arXiv:2503.24004 source file (2026-02-02)
Supplement: Supplementary file 1 [file supp.pdf]

# Supplementary Materials for Multivariate Species Sampling Models

Beatrice Franzolini, Antonio Lijoi, Igor Prünster

Bocconi Institute for Data Science and Analytics, Bocconi University, Italy

Giovanni Rebaudo

ESOMAS Dept., University of Torino and Collegio Carlo Alberto, Italy

## S.1 Some basics on (univariate) species sampling

In classical species sampling problems, a random sample  $(X_1, \dots, X_n)$  is extracted from an unknown and typically discrete distribution and each observed value corresponds to the species of a drawn individual. Denoting with  $P$  the unknown distribution of species in the population we have

$$X_i \mid P \stackrel{iid}{\sim} P \quad \text{for } i = 1, \dots, n.$$

To develop a Bayesian model for species sampling problems, a prior must be defined over the unknown distribution  $P$ . In the univariate setting, the problem can be tackled relying on the large class of priors provided by species sampling processes (SSP), introduced by Pitman (1996) as a generalization of the Dirichlet process of Ferguson (1973).

**Definition 1** (SSP). *A random probability measure  $P$  is a species sampling process (SSP) if*

$$P \stackrel{a.s.}{=} \sum_{h \geq 1} \pi_h \delta_{\theta_h} + \left(1 - \sum_{h \geq 1} \pi_h\right) P_0,$$

where the atoms  $(\theta_h)_{h \geq 1}$  are i.i.d. from the non-atomic distribution  $P_0$  and are independent of the random sub-probability vector of the weights  $\boldsymbol{\pi} = (\pi_h)_h$ . Moreover, if  $\sum_{h \geq 1} \pi_h \stackrel{a.s.}{=} 1$ ,  $P$  is said proper.

The corresponding model is defined once the observations are sampled independently from  $P$  given  $P$ .

**Definition 2** (SSM). *An infinite sequence of random variables  $X_1, X_2, \dots$  follows a species sampling model (SSM) if it is exchangeable with an SSP directing measure. That is*

$$\begin{aligned} X_i \mid P &\stackrel{iid}{\sim} P \quad (i = 1, 2, \dots) \\ P &\sim \text{SSP}(\mathcal{L}_\pi, P_0). \end{aligned} \tag{S.1}$$

Any sample  $(X_1, \dots, X_n)$  arising from a  $P \sim \text{SSP}(\mathcal{L}_\pi, P_0)$  induces a random partition of the labels of the observations in the sample, i.e., of  $[n] = \{1, \dots, n\}$ . More precisely, two observation labels  $i$  and  $l$  belong to the same block of the partition of  $[n]$  (i.e.,  $X_i$  and  $X_l$  are clustered together) if and only if  $X_i = X_l$ . The discrete part of the SSP entails that two observations are clustered together with positive probability since  $\mathbb{P}(X_i = X_l) > 0$ . The law of such a random partition (denoted  $\Pi_n$ ) of  $[n]$  is characterized by the exchangeable partition probability functions (EPPF) (Pitman, 1996).

More precisely, let  $\{C_1, \dots, C_K\}$  an arbitrary partition of  $[n]$  for a given  $n \in \mathbb{N}$  and  $n_k = |C_k|$  for  $k \in [K]$  then

$$\mathbb{P}(\Pi_n = \{C_1, \dots, C_K\}) = \text{EPPF}_K^{(n)}(n_1, \dots, n_K). \quad (\text{S.2})$$

In words,  $\text{EPPF}_K^{(n)}(n_1, \dots, n_K)$  can be interpreted as the probability of observing a particular (unordered) partition of  $n$  observations into  $K$  subsets of cardinalities  $\{n_1, \dots, n_K\}$ . Note that, the EPPF is defined on the space of the compositions of  $n$ , which can be interpreted as the space of the frequency of the partition in a given arbitrary order (e.g., the order of arrival). Let  $P = \sum_{h \geq 1} \pi_h \delta_{\theta_h}$  be a proper SSP. Then the induced EPPF can be computed as

$$\text{EPPF}_K^{(n)}(n_1, \dots, n_K) = \mathbb{E} \left[ \sum_{h_1 \neq \dots \neq h_j} \prod_{k=1}^K \pi_{h_k}^{n_k} \right]. \quad (\text{S.3})$$

The EPPF characterizes the SSM (Pitman, 1996). For any  $n \in \mathbb{N}$ , if  $(X_1, \dots, X_n)$  arises from an SSM, its law can be obtained hierarchically as

1. sample the random partition  $\Pi_n$  from the induced EPPF obtained as in (S.3);
2. sample iid the unique values associated with each set in the partition from  $P_0$ .

The EPPF and the SSP can also be characterized by a specific sequence of predictive distributions (Pitman, 1996) also known as the *generalized Chinese restaurant process* (gCRP). In the culinary metaphor, we can think of observations corresponding to customers in a restaurant, they arrive sequentially and sit at an already occupied table or a new table and each table serves a different dish (iid sampled from  $P_0$ ).

It is theoretically straightforward to derive the predictive distribution associated with any SSP via ratios of EPPFs as an application of the definition of conditional probability, leading to

$$\mathbb{P}(X_{n+1} = x \mid \mathbf{X}) = \begin{cases} \frac{\text{EPPF}_K^{(n+1)}(n_1, \dots, n_k+1, \dots, n_K)}{\text{EPPF}_K^{(n)}(n_1, \dots, n_k, \dots, n_K)} & \text{if } x = X_k^* \quad \text{and } k = 1, \dots, K \\ \frac{\text{EPPF}_{K+1}^{(n+1)}(n_1, \dots, n_k, \dots, n_K, 1)}{\text{EPPF}_K^{(n)}(n_1, \dots, n_k, \dots, n_K)} & \text{if } x = X_{K+1}^*, \end{cases} \quad (\text{S.4})$$

where  $(X_k^* : k = 1, \dots, K)$  denote the  $K$  unique values of  $X_1, \dots, X_n$  that were recorded with frequency  $n_1, \dots, n_K$  and are iid sampled from  $P_0$ . See Pitman (1996, 2006); Lee *et al.* (2013);

Ghosal and van der Vaart (2017) for details and proofs about different characterizations of (univariate) SSM.

Although the analytical expression of the gCRP is available from the EPPF as shown in (S.4), such expression does not reduce to simple and tractable quantities in general. However, a notable exception is the subclass of Gibbs-type prior (Gnedin and Pitman, 2006; De Blasi *et al.*, 2015), which thanks to the product partition form of the EPPF allows the ratio of EPPF in the gCRP to boil down to a simple ratio of constant for several notable examples as in the well known Chinese restaurant franchise (CRP) (Blackwell and MacQueen, 1973) induced by the Dirichlet process (DP) (Ferguson, 1973). The class of Gibbs-type prior is the most natural tractable generalization of the DP (De Blasi *et al.*, 2015) and it includes the symmetric finite Dirichlet prior (Green and Richardson, 2001), the Pitman-Yor process (PYP) (Pitman and Yor, 1997), the normalized inverse Gaussian (NIG) (Lijoi *et al.*, 2005), the normalized generalized gamma process (NGGP) (Lijoi *et al.*, 2007), mixture of finite symmetric Dirichlet (Nobile, 1994; Richardson and Green, 1997; Nobile and Fearnside, 2007; Miller and Harrison, 2018) and the mixture of DP (MDP) models (Antoniak, 1974). In the following sections, we recall the analytical expression of the three different characterizations (i.e., SSP, EPPF, and gCRP) of some relevant and tractable examples of Gibbs-type prior commonly used in Bayesian analysis.

### S.1.1 Pitman-Yor process (PYP)

We say that an SSP( $\mathcal{L}_\pi, P_0$ ) follow a Pitman-Yor process, i.e.,  $P \sim \text{PYP}(\alpha, \gamma; P_0)$ , with  $P_0$  a non-atomic measure if it is a proper SSP with  $\mathcal{L}_\pi \sim \text{GEM}(\alpha, \gamma)$ , where the two parameters GEM distribution, named after Griffiths, Engen, and McCloskey, can be thought as arising from the stick-breaking construction where the  $\pi_i$ 's are such that  $\pi_i = v_i \prod_{l=1}^{i-1} v_l$ , with  $v_i \sim \text{BETA}(1 - \alpha, \gamma + i\alpha)$ ,  $i \geq 1$ ,  $\alpha \in [0, 1)$  and  $\gamma > -\alpha$ .

The following EPPF characterizes the PYP

$$\text{EPPF}_K^{(n)}(n_1, \dots, n_K; \alpha, \gamma) = \frac{\prod_{k=1}^{K-1} (\gamma + k\alpha)}{(\gamma + 1)_{n-1}} \prod_{k=1}^K (1 - \alpha)_{n_k-1}, \quad (\text{S.5})$$

where  $(x)_n = x(x+1) \cdots (x+n-1)$  is the  $n$ th ascending factorial.

Denoting with  $X_1, X_2, \dots$  an SSM from  $P \sim \text{PYP}(\alpha, \gamma; P_0)$ , we can derive the well-known gCRP of the PYP from the EPPF in (S.5) applying the definition of conditional probability.

$$\mathbb{P}(X_{n+1} = x \mid \mathbf{X}) = \begin{cases} \frac{n_k - \alpha}{\gamma + n} & \text{if } x = X_k^* \quad \text{and } k = 1, \dots, K \\ \frac{\gamma + \alpha K}{\gamma + n} & \text{if } x = X_{K+1}^*. \end{cases} \quad (\text{S.6})$$

### S.1.2 Dirichlet process (DP)

If we consider  $P \sim \text{PYP}(\alpha, \gamma; P_0)$  as in the previous section and we restrict  $\alpha = 0$  and  $\gamma > 0$  we obtain the relevant special case of the Dirichlet process, i.e.,  $P \sim \text{DP}(\gamma; P_0)$ . Thus we

can specialize the distribution of the weights to  $\text{GEM}(\gamma)$ , the induced EPFF in (S.5) that boils down to

$$\text{EPPF}_K^{(n)}(n_1, \dots, n_K; \alpha, \gamma) = \frac{\gamma^K \Gamma(\gamma)}{\Gamma(\gamma + n)} \prod_{k=1}^K (n_k - 1)!, \quad (\text{S.7})$$

and the corresponding CRP

$$\mathbb{P}(X_{n+1} = x \mid \mathbf{X}) = \begin{cases} \frac{n_k}{\gamma + n} & \text{if } x = X_k^* \quad \text{and } k = 1, \dots, K \\ \frac{\gamma}{\gamma + n} & \text{if } x = X_{K+1}^*. \end{cases} \quad (\text{S.8})$$

### S.1.3 Finite symmetric Dirichlet multinomial (symDM)

Here we consider an SSP  $P$  with a fixed known number  $M$  of species in the population (with  $M \in \mathbb{N}$ ) that follow a finite-dimensional symmetric Dirichlet multinomial (symDM). That is, for a fixed  $M \in \mathbb{N}$ ,

$$P = \sum_{h=1}^M \pi_h \delta_{\theta_h}, \quad (\text{S.9})$$

where  $(\pi_1, \dots, \pi_M) \sim \text{Dir}(\rho, \dots, \rho) \perp \theta_h \stackrel{\text{iid}}{\sim} P_0$ . We write  $P \sim \text{DM}_M(\rho, P_0)$ .

Then we can derive the induced EPFF as

$$\text{EPPF}_K^{(n)}(n_1, \dots, n_K) = \frac{M!}{(M - K)!} \frac{\Gamma(\rho M)}{\Gamma(n + \rho M) \Gamma(\rho)^K} \prod_{k=1}^K \Gamma(n_k + \rho). \quad (\text{S.10})$$

and the corresponding gCRP

$$\mathbb{P}(X_{n+1} = x \mid \mathbf{X}) \propto \begin{cases} n_k + \rho & \text{if } x = X_k^* \quad \text{and } k = 1, \dots, K \\ \rho(M - K) \mathbf{1}(K \neq M) & \text{if } x = X_{K+1}^*. \end{cases} \quad (\text{S.11})$$

### S.1.4 Gnedin Process (GN)

Allowing for unknown  $M$  in finite-dimensional symmetric Dirichlet multinomial process, the model becomes a mixture of symmetric Dirichlet models. A relevant example is the *Gnedin process* (with discount parameter equals to  $-1$ ). The corresponding EPFF is

$$\text{EPPF}_K^{(n)}(n_1, \dots, n_K) = \sum_{m=1}^{\infty} \text{EPPF}_K^{(n)}(n_1, \dots, n_K \mid M = m) p(M = m), \quad (\text{S.12})$$

where  $\text{EPPF}_K^{(n)}(n_1, \dots, n_K \mid M = m)$  is the EPPF of the  $M$ -symmetric Dirichlet prior in (S.10), with  $\rho = 1$  and  $p(M = m) = \frac{\gamma(1-\gamma)^{m-1}}{m!}$ ,  $\gamma \in (0, 1)$ .

The corresponding gCRP boils down to the following simple tractable expression

$$\mathbb{P}(X_{n+1} = x \mid \mathbf{X}) \propto \begin{cases} (n_k + 1)(n - K + \gamma) & \text{if } x = X_k^* \quad \text{and } k = 1, \dots, K \\ K^2 - K\gamma & \text{if } x = X_{K+1}^*. \end{cases} \quad (\text{S.13})$$

We denote the corresponding SSP with  $P \sim \text{GN}(\gamma, P_0)$ .

## S.2 Proofs

### S.2.1 Proof of Proposition 1

The proof follows trivially from the Definition of mSSP.

### S.2.2 Proof of Proposition 2

*Proof.* To prove the statement we want to show the non-trivial implication of the iff, i.e., if  $(P_1, P_2)$  are a mSSP with non-atomic base measure  $P_0$  they can be rewritten as in (1), that is

$$P_j \stackrel{\text{a.s.}}{=} \sum_{h \geq 1} \pi_{j,h}^{(1,2)} \delta_{\theta_{0,h}} + \sum_{h' \geq 1} \pi_{j,h'}^{(j)} \delta_{\theta_{j,h'}} + \pi_{j,0}^{(j)} P_0, \quad \text{for } j = 1, 2. \quad (\text{S.14})$$

where  $\sum_{h \geq 1} \pi_{j,h}^{(1,2)} + \sum_{h' \geq 0} \pi_{j,h'}^{(j)} = 1$ , for  $j = 1, 2$ , the atoms are independent from the weights and such that  $\theta_{j,h} \stackrel{\text{iid}}{\sim} P_0$ , for  $j = 0, 1, 2$ ,  $h = 1, 2, \dots$  and  $\mathbb{P}[\pi_{1,h}^{(1,2)} > 0, \pi_{2,h}^{(1,2)} > 0] > 0$ .

From the definition of mSSP, we write for  $j = 1, 2$

$$P_j = \sum_{h \geq 1} \pi_{j,h} \delta_{\theta_h} + \left(1 - \sum_{h \geq 1} \pi_{j,h}\right) P_0 = \sum_{h \in \mathcal{H}} \pi_{j,h} \delta_{\theta_h} + \left(1 - \sum_{h \in \mathcal{H}} \pi_{j,h}\right) P_0,$$

where we denote by  $\mathcal{H} := \{1, 2, \dots\}$  the set of the indexes of the two sums. Note that  $H := \text{card}(\mathcal{H}) \in \{0\} \cup \mathbb{N} \cup \{\infty\}$ , and we use the convention that, for any  $(x_h)_h$ ,  $\sum_{h=1}^0 x_h = \sum_{h \in \emptyset} x_h = 0$ . We define  $\pi_{j,0}^{(j)} := 1 - \sum_{h \in \mathcal{H}} \pi_{j,h}$  and we partition  $\mathcal{H}$  in  $\{\mathcal{H}_0, \bar{\mathcal{H}}_0\}$ , where

$$\mathcal{H}_0 := \{h \in \mathcal{H} : \Pr[\pi_{1,h} > 0, \pi_{2,h} > 0] > 0\} = \{h \in \mathcal{H} : \Pr[\pi_{1,h} \pi_{2,h} > 0] > 0\}$$

is the set of shared atoms and  $\bar{\mathcal{H}}_0 = \mathcal{H} \setminus \mathcal{H}_0$ .

Let us define, for  $j = 1, 2$ ,

$$\left( (\theta_{0,h}, \pi_{j,h}^{(12)}) : h \in \mathcal{H}_0 \right) := ((\theta_h, \pi_{j,h}) : h \in \mathcal{H}_0) \text{ and } \left( \pi_{j,h}^{(j)} : h \in \bar{\mathcal{H}}_0 \right) := (\pi_{j,h} : h \in \bar{\mathcal{H}}_0),$$

and  $\theta_{j,h} \stackrel{\text{iid}}{\sim} P_0$ , for  $j = 1, 2$  and  $h \in \bar{\mathcal{H}}_0$ , independent from all the previous random variables, i.e.,  $\left( (\theta_{0,h}, \pi_{j,h}^{(12)}) : h \in \mathcal{H}_0 \right)$  and  $\left( \pi_{j,h}^{(j)} : h \in \bar{\mathcal{H}}_0 \right)$ .

Then note that, for  $j = 1, 2$ ,

$$\sum_{h \in \mathcal{H}} \pi_{j,h} \delta_{\theta_h} = \sum_{h \in \mathcal{H}_0} \pi_{j,h} \delta_{\theta_h} + \sum_{h \in \bar{\mathcal{H}}_0} \pi_{j,h} \delta_{\theta_h}$$

and

$$\sum_{h \in \mathcal{H}_0} \pi_{j,h} \delta_{\theta_h} = \sum_{h \in \mathcal{H}_0} \pi_{j,h}^{(12)} \delta_{\theta_{0,h}} \text{ and } \sum_{h \in \bar{\mathcal{H}}_0} \pi_{j,h} \delta_{\theta_h} = \sum_{h \in \bar{\mathcal{H}}_0} \pi_{j,h}^{(j)} \delta_{\theta_{j,h}}.$$

To conclude the proof we just relabel the indexes in both  $\mathcal{H}_0$  and  $\bar{\mathcal{H}}_0$  such that they are ordered integers starting from 1 with no gaps and remap the elements in the corresponding sums accordingly. □

### S.2.3 Proof of Proposition 3

*Proof.* By the law of iterated expectations, the first and second moments of  $P_j(A)$  are equal to

$$\mathbb{E}[P_j(A)] = \mathbb{P}(X_{j,i} \in A) = P_0(A) \quad \text{and} \quad \mathbb{E}[P_j(A)^2] = \mathbb{P}(X_{j,i} \in A, X_{j,l} \in A), \text{ with } i \neq l.$$

Disintegrating with respect to  $\{X_{j,i} = X_{j,l}\}$  to recover independence leads to

$$\begin{aligned} \mathbb{P}(X_{j,i} \in A, X_{j,l} \in A) &= \mathbb{P}(X_{j,i} = X_{j,l}) \mathbb{P}(X_{j,i} \in A, X_{j,l} \in A \mid X_{j,i} = X_{j,l}) \\ &\quad + \mathbb{P}(X_{j,i} \neq X_{j,l}) \mathbb{P}(X_{j,i} \in A, X_{j,l} \in A \mid X_{j,i} \neq X_{j,l}) \\ &= \mathbb{P}(X_{j,i} = X_{j,l}) P_0(A) + \mathbb{P}(X_{j,i} \neq X_{j,l}) P_0(A)^2. \end{aligned}$$

Finally,  $\text{Var}[P_j(A)] = \mathbb{E}[P_j(A)^2] - \mathbb{E}[P_j(A)]^2 = \mathbb{P}(X_{j,i} = X_{j,l}) P_0(A) [1 - P_0(A)]$ . □

### S.2.4 Proof of Proposition 4

*Proof.* For  $j \neq k$ , by the law of iterated expectations, we get

$$\mathbb{E}[P_j(A)P_k(A)] = \mathbb{P}(X_{j,i} \in A, X_{k,m} \in A).$$

Disintegrating with respect to  $\{X_{j,i} = X_{k,m}\}$  to recover independence leads to

$$\begin{aligned} \mathbb{P}(X_{j,i} \in A, X_{k,m} \in A) &= \mathbb{P}(X_{j,i} = X_{k,m})\mathbb{P}(X_{j,i} \in A, X_{k,m} \in A \mid X_{j,i} = X_{k,m}) \\ &\quad + \mathbb{P}(X_{j,i} \neq X_{k,m})\mathbb{P}(X_{j,i} \in A, X_{k,m} \in A \mid X_{j,i} \neq X_{k,m}) \\ &= \mathbb{P}(X_{j,i} = X_{k,m})P_0(A) + \mathbb{P}(X_{j,i} \neq X_{k,m})P_0(A)^2. \end{aligned}$$

Thus,  $\text{Cov}[P_j(A), P_k(A)] = \mathbb{P}(X_{j,i} = X_{k,m})P_0(A)[1 - P_0(A)]$ . The correlation is obtained using Proposition 3.  $\square$

### S.2.5 Proof of Proposition 5

*Proof.* By definition of mSSP, we know that

$$P_j \stackrel{a.s.}{=} \sum_{h \geq 1} \pi_{j,h} \delta_{\theta_h} + \left(1 - \sum_{h \geq 1} \pi_{j,h}\right) P_0 \quad \text{and} \quad P_k \stackrel{a.s.}{=} \sum_{h \geq 1} \pi_{k,h} \delta_{\theta_h} + \left(1 - \sum_{h \geq 1} \pi_{k,h}\right) P_0.$$

Moreover, by Cauchy-Schwarz inequality we have a.s. that

$$\begin{aligned} &\sqrt{\sum_{h \geq 1} \pi_{j,h}^2 + \left(1 - \sum_{h \geq 1} \pi_{j,h}\right)^2} \sqrt{\sum_{h \geq 1} \pi_{k,h}^2 + \left(1 - \sum_{h \geq 1} \pi_{k,h}\right)^2} \\ &\geq \sum_{h \geq 1} \pi_{j,h} \pi_{k,h} + \left(1 - \sum_{h \geq 1} \pi_{j,h}\right) \left(1 - \sum_{h \geq 1} \pi_{k,h}\right). \end{aligned}$$

Assume by contradiction that the event  $\{\pi_{j,h} \neq \pi_{k,h} \text{ for at least one } h\}$  has positive probability. This implies that with positive probability the above inequality is strict and thus, with positive probability we have

$$\mathbb{P}(X_{j,1} = X_{k,1} \mid P_j, P_k) < \sqrt{\mathbb{P}(X_{j,1} = X_{j,2} \mid P_j, P_k)} \sqrt{\mathbb{P}(X_{k,1} = X_{k,2} \mid P_j, P_k)}$$

which implies  $\mathbb{P}(X_{j,1} = X_{k,1}) < \mathbb{P}(X_{j,1} = X_{j,2})\mathbb{P}(X_{k,1} = X_{k,2})$  and  $\text{Cor}[P_j(A), P_k(A)] < 1$ . Therefore, we have  $\pi_{j,h} = \pi_{k,h}$  a.s., for all  $h$ , and thus  $P_j \stackrel{a.s.}{=} P_k$ .  $\square$

### S.2.6 Proof of Theorem 1

*Proof.* Clearly  $P_j \perp P_k$  entails  $\text{Cor}[P_j(A), P_k(A)] = 0$ . We want to show that  $\text{Cor}[P_j(A), P_k(A)] = 0$  entails  $P_j \perp P_k$ .

Let us consider the representation of  $(P_j, P_k)$  as mixtures of two components

$$P_j \stackrel{a.s.}{=} \omega_j^{(j,k)} \sum_{h \geq 1} \bar{\pi}_{j,h}^{(j,k)} \delta_{\theta_h} + \left(1 - \omega_j^{(j,k)}\right) \left( \bar{\pi}_{j,0}^{(j)} P_0 + \sum_{h' \geq 1} \bar{\pi}_{j,h'}^{(j)} \delta_{\theta_{j,h'}} \right)$$

and

$$P_k \stackrel{a.s.}{=} \omega_k^{(j,k)} \sum_{h \geq 1} \bar{\pi}_{k,h}^{(j,k)} \delta_{\theta_h} + \left(1 - \omega_k^{(j,k)}\right) \left( \bar{\pi}_{j,0}^{(k)} P_0 + \sum_{h' \geq 1} \bar{\pi}_{k,h'}^{(k)} \delta_{\theta_{k,h'}} \right).$$

where  $\bar{\pi}_{j,h}^{(j,k)} = \frac{\pi_{j,h}^{(j,k)}}{\sum_{\ell \geq 1} \pi_{j,\ell}^{(j,k)}}$ ,  $\bar{\pi}_{j,h'}^{(j)} = \frac{\pi_{j,h'}^{(j)}}{\sum_{\ell \geq 0} \pi_{j,\ell}^{(j)}}$ , and  $\omega_j^{(j,k)} = \sum_{h \geq 1} \pi_{j,h}^{(j,k)}$ . Recall that by Proposition 4,  $\text{Cor}[P_j(A), P_k(A)] = 0$  iff  $\mathbb{P}(X_{1,j} = X_{1,k}) = 0$ .

Note that

$$\mathbb{P}(X_{j,1} = X_{k,1}) = \sum_{h \geq 1} \mathbb{E} \left[ \omega_j^{(j,k)} \bar{\pi}_{j,h}^{(j,k)} \omega_k^{(j,k)} \bar{\pi}_{k,h}^{(j,k)} \right] \geq \mathbb{E} \left[ \omega_j^{(j,k)} \bar{\pi}_{j,1}^{(j,k)} \omega_k^{(j,k)} \bar{\pi}_{k,1}^{(j,k)} \right].$$

Therefore, by Definition of rmSSP, we have that  $\omega_j^{(j,k)} \stackrel{a.s.}{=} \omega_k^{(j,k)} \stackrel{a.s.}{=} 0$ .

Indeed, if we assume by contradiction that (w.l.o.g.)  $\mathbb{P}(\omega_j^{(j,k)} > 0) > 0$  than by Definition 3 we have that  $\mathbb{P}(\omega_j^{(j,k)} \bar{\pi}_{j,1}^{(j,k)} \omega_k^{(j,k)} \bar{\pi}_{k,1}^{(j,k)} > 0) > 0$  that entails

$$\mathbb{P}(X_{j,1} = X_{k,1}) \geq \mathbb{E} \left[ \omega_j^{(j,k)} \bar{\pi}_{j,1}^{(j,k)} \omega_k^{(j,k)} \bar{\pi}_{k,1}^{(j,k)} \right] > 0$$

that contradicts  $\mathbb{P}(X_{1,j} = X_{1,k}) = 0$ . Since  $\omega_j^{(j,k)} \stackrel{a.s.}{=} \omega_k^{(j,k)} \stackrel{a.s.}{=} 0$  we can rewrite

$$P_j \stackrel{a.s.}{=} \bar{\pi}_{j,0}^{(j)} P_0 + \sum_{h' \geq 1} \bar{\pi}_{j,h'}^{(j)} \delta_{\theta_{j,h'}}$$

and

$$P_k \stackrel{a.s.}{=} \bar{\pi}_{j,0}^{(k)} P_0 + \sum_{h' \geq 1} \bar{\pi}_{k,h'}^{(k)} \delta_{\theta_{k,h'}}$$

and therefore  $P_j \perp P_k$ . □



### S.2.7 Proof of Proposition 6

*Proof.* Define the random variable  $Z$ , so that  $Z = 1$ , if  $X_{j,i} = X_{k,m}$ , and  $Z = 0$ , otherwise.

$$\begin{aligned}
 \text{Cov}(X_{j,i}, X_{k,m}) &= \mathbb{E}[\text{Cov}(X_{j,i}, X_{k,m} \mid Z)] + \text{Cov}(\mathbb{E}[X_{j,i} \mid Z], \mathbb{E}[X_{k,m} \mid Z]) \\
 &= \mathbb{E}[\text{Cov}(X_{j,i}, X_{k,m} \mid Z)] + 0 \\
 &= \text{Cov}(X_{j,i}, X_{k,m} \mid Z = 1)\mathbb{P}(X_{j,i} = X_{k,m}) \\
 &= \mathbb{P}(X_{j,i} = X_{k,m})\text{Var}(X^*).
 \end{aligned}$$

where  $X^* \sim P_0$ . □

### S.2.8 Proof of Proposition 7

*Proof.* Define  $\mathbf{X}_{j,1:q} = (X_{j,1}, \dots, X_{j,q})$ ,

$$\mathbb{E}[P_j(A)^q] = \mathbb{P}(\mathbf{X}_{j,1:q} \in A^q).$$

Disintegrate with respect to the random partition  $\Pi_q^{(j)}$  induced by the ties in  $\mathbf{X}_{j,1:q}$  and taking values in the set  $\mathcal{P}(\mathbf{X}_{j,1:q})$  to recover independence and aggregate by symmetry induced by exchangeability.  $K_q^{(j)}$  denotes the number of sets in  $\Pi_q^{(j)}$ .

$$\begin{aligned}
 &\sum_{\Pi_q^{(j)} \in \mathcal{P}(\mathbf{X}_{j,1:q})} \mathbb{P}[\mathbf{X}_{j,1:q} \in A^q \mid \Pi_q^{(j)}] \mathbb{P}(\Pi_q^{(j)}) = \\
 &= \sum_{s=1}^q P_0(A)^s \sum_{\Pi_q^{(j)} \in \mathcal{P}(\mathbf{X}_{j,1:q}): K_q^{(j)}=s} \mathbb{P}(\Pi_q^{(j)}) = \\
 &= \sum_{s=1}^q P_0(A)^s \mathbb{P}(K_q^{(j)} = s) = \mathbb{E}[P_0(A)^{K_q^{(j)}}].
 \end{aligned}$$

□

### S.2.9 Proof of Proposition 8

*Proof.* For notational convenience, we prove the proposition for  $h = 2$ . The general case can be proven with the same argument. Notation is the same as in the proof of Proposition 7.

$$\mathbb{E}[P_j(A_1)^{q_1} P_j(A_2)^{q_2}] = \mathbb{P}[\mathbf{X}_{j,1:q} \in A_1^{q_1} \times A_2^{q_2}],$$

where  $q = q_1 + q_2$ . Denote now with  $\mathcal{A}_{q_1, q_2} \subset \mathcal{P}(\mathbf{X}_{j, 1:q})$  the set of all possible partitions  $\Pi_q^{(j)}$  induced by the ties in  $\mathbf{X}_{j, 1:q}$  such that the elements in  $\mathbf{X}_{j, 1:q_1}$  and in  $\mathbf{X}_{j, q_1+1:q_2}$  do not have ties. It follows that

$$\begin{aligned}
\mathbb{P}[\mathbf{X}_{j, 1:q} \in A_1^{q_1} \times A_2^{q_2}] &= \mathbb{P}[(\mathbf{X}_{j, 1:q} \in A_1^{q_1} \times A_2^{q_2}) \cap (\Pi_q^{(j)} \in \mathcal{A}_{q_1, q_2})] = \\
&= \sum_{s_1=1}^{q_1} \sum_{s_2=1}^{q_2} \mathbb{P}(\Pi_q^{(j)} \in \mathcal{A}_{q_1, q_2}, K_{q_1}^{(j)} = s_1, K_{q_1+1:q_2}^{(j)} = s_2) \times \\
&\quad \times \mathbb{P}(\mathbf{X}_{j, 1:q} \in A_1^{q_1} \times A_2^{q_2} \mid \Pi_q^{(j)} \in \mathcal{A}_{q_1, q_2}, K_{q_1}^{(j)} = s_1, K_{q_1+1:q_2}^{(j)} = s_2) = \\
&= \sum_{s_1=1}^{q_1} \sum_{s_2=1}^{q_2} P_0(A_1)^{s_1} P_0(A_2)^{s_2} \mathbb{P}(\Pi_q^{(j)} \in \mathcal{A}_{q_1, q_2}, K_{q_1}^{(j)} = s_1, K_{q_1+1:q_2}^{(j)} = s_2) \\
&= \mathbb{E} \left[ P_0(A_1)^{K_{q_1}^{(j)}} P_0(A_2)^{K_{q_1+1:q_2}^{(j)}} \mid \Pi_q^{(j)} \in \mathcal{A}_{q_1, q_2} \right] \mathbb{P}(\Pi_q^{(j)} \in \mathcal{A}_{q_1, q_2}).
\end{aligned}$$

□

## S.2.10 Proof of Theorem 2

*Proof.*

$$\mathbb{E}[P_1(A)^{q_1} \cdots P_J(A)^{q_J}] = \mathbb{P}(\mathbf{X}_{j, 1:q_j} \in A^{q_j} : j = 1, \dots, J).$$

Disintegrate with respect to the possible partitions  $\Pi_q$  of  $\mathbf{X}_{1:q_1, \dots, 1:q_J}$  to recover independence and aggregate by symmetry.

$$\begin{aligned}
&\sum_{\Pi_q \in \mathcal{P}(\mathbf{X}_{1:q_1, \dots, 1:q_J})} \mathbb{P}(\mathbf{X}_{j, 1:q_j} \in A^{q_j} : j = 1, \dots, J \mid \Pi_q) \mathbb{P}(\Pi_q) = \\
&= \sum_{s=1}^q P_0(A)^s \sum_{\Pi_q \in \mathcal{P}(\mathbf{X}_{1:q_1, \dots, 1:q_J}) : K_{q_1, \dots, q_J} = s} \mathbb{P}(\Pi_q) \\
&= \sum_{s=1}^q P_0(A)^s \mathbb{P}(K_{q_1, \dots, q_J} = s) = \mathbb{E}[P_0(A)^{K_{q_1, \dots, q_J}}].
\end{aligned}$$

□

### S.2.11 Proof of Theorem 3

*Proof.* First note that

$$\mathbb{E} \left( \prod_{j=1}^J P_j(A_j)^{q_j} \right) = \mathbb{P} \left( \mathbf{X}_{1:q_1, \dots, 1:q_J} \in \bigtimes_{j=1}^J A_j^{q_j} \right).$$

Denote now with  $\mathcal{A}_{q_1, \dots, q_J} \subset \mathcal{P}(\mathbf{X}_{1:q_1, \dots, 1:q_J})$  the set of all possible partitions  $\Pi_q$  of the elements in  $\mathbf{X}_{1:q_1, \dots, 1:q_J}$  such that the elements in  $\mathbf{X}_{j, 1:q_1}$  and in  $\mathbf{X}_{j', 1:q_{j'}}$  do not belong to the same set, for any  $j \neq j'$  according to  $\Pi_q$ .

$$\begin{aligned} \mathbb{P} \left( \mathbf{X}_{1:q_1, \dots, 1:q_J} \in \bigtimes_{j=1}^J A_j^{q_j} \right) &= \mathbb{P} \left[ \left( \mathbf{X}_{1:q_1, \dots, 1:q_J} \in \bigtimes_{j=1}^J A_j^{q_j} \right) \cap (\Pi_q \in \mathcal{A}_{q_1, \dots, q_J}) \right] = \\ &= \mathbb{P}(\Pi_q \in \mathcal{A}_{q_1, \dots, q_J}) \mathbb{P} \left( \mathbf{X}_{1:q_1, \dots, 1:q_J} \in \bigtimes_{j=1}^J A_j^{q_j} \mid \Pi_q \in \mathcal{A}_{q_1, \dots, q_J} \right) = \\ &= \sum_{s_1=1}^{q_1} \cdots \sum_{s_J=1}^{q_J} \mathbb{P}(\Pi_q \in \mathcal{A}_{q_1, \dots, q_J}, K_{q_1}^{(1)} = s_1, \dots, K_{q_J}^{(J)} = s_J) \times \\ &\quad \times \mathbb{P} \left( \mathbf{X}_{1:q_1, \dots, 1:q_J} \in \bigtimes_{j=1}^J A_j^{q_j} \mid \Pi_q \in \mathcal{A}_{q_1, \dots, q_J}, K_{q_1}^{(1)} = s_1, \dots, K_{q_J}^{(J)} = s_J \right) = \\ &= \sum_{s_1=1}^{q_1} \cdots \sum_{s_J=1}^{q_J} P_0(A_1)^{s_1} \cdots P_0(A_J)^{s_J} \times \\ &\quad \times \mathbb{P}(\Pi_q \in \mathcal{A}_{q_1, \dots, q_J}, K_{q_1}^{(1)} = s_1, \dots, K_{q_J}^{(J)} = s_J) \\ &= \mathbb{E} \left[ P_0(A_1)^{K_{q_1}^{(1)}} \cdots P_0(A_J)^{K_{q_J}^{(J)}} \mid \Pi_q \in \mathcal{A}_{q_1, \dots, q_J} \right] \mathbb{P}(\Pi_q \in \mathcal{A}_{q_1, \dots, q_J}). \end{aligned}$$

□

### S.2.12 Proof of Proposition 9

*Proof.*

$$\begin{aligned} \text{pEPPF}_D^{(n)}(\mathbf{n}_1, \dots, \mathbf{n}_J) &= \mathbb{E} \left[ \int_{\mathbb{X}_*^D} \prod_{d=1}^D P_1(\mathrm{d}x_d)^{n_{1,d}} \cdots P_J(\mathrm{d}x_d)^{n_{J,d}} \right] \\ &= \mathbb{E} \left\{ \int_{\mathbb{X}_*^D} \prod_{d=1}^D \prod_{j=1}^J \left[ \sum_{h \geq 1} \pi_{j,h} \delta_{\theta_h}(\mathrm{d}x_d) \right]^{n_{j,d}} \right\} = \mathbb{E} \left[ \sum_{h_1 \neq \dots \neq h_D} \prod_{j=1}^J \prod_{d=1}^D \pi_{j,h_d}^{n_{j,d}} \right]. \end{aligned}$$

□

### S.2.13 Proof of Theorem 4

*Proof.* For any family of sets  $(A_{j,i} : i \in [I_j], j \in [J])$ ,

$$\begin{aligned}
& \mathbb{P}[(X_{j,i} : i \in [I_j], j \in [J]) \in (A_{j,i} : i \in [I_j], j \in [J])] \\
&= \sum_{\Pi_n \in \mathbb{P}[\Pi_n] \mathcal{P}(\mathbf{X}_{1:I_1, \dots, 1:I_J})} \mathbb{P}[(X_{j,i} : i \in [I_j], j \in [J]) \in (A_{j,i} : i \in [I_j], j \in [J]) \mid \Pi_n] \\
&= \sum_{\substack{\{C_1, \dots, C_D\} \\ \in \mathcal{P}(\mathbf{X}_{1:I_1, \dots, 1:I_J})}} \mathbb{P}[\Pi_n = \{C_1, \dots, C_D\}] \prod_{d=1}^D P_0 \left( \bigcap_{(j,i): \sum_{j'=1}^{j-1} I_{j'} + i \in C_d} A_{j,i} \right)
\end{aligned}$$

where  $C_1, \dots, C_D$  are the set in  $\Pi_n$ , whose elements are collected according to the order of arrival by groups.  $\square$

### S.2.14 Proof of Proposition 10

The proof follows trivially by the definition of conditional probability.

## S.3 Algorithms and models details for the multi-armed bandit illustration

The algorithms used for all six strategies considered in Section 6 are Markov chain Monte Carlo marginal algorithms. These algorithms are obtained using the augmented representation of the pEPPF described in Section 5 for the additive and hierarchical processes, and the sequential sampling schemes detailed in Section S1 for the independent processes. All models are generalized to accommodate random hyperparameters to achieve greater flexibility in the learning mechanisms, leading to the following specifications for the six strategies.

- Independent Dirichlet Process

$$\begin{aligned}
X_{j,i} \mid (P_1, \dots, P_J) &\stackrel{\text{ind}}{\sim} P_j \quad \text{for } i = 1, 2, \dots \\
P_j \mid \alpha_j &\stackrel{\text{ind}}{\sim} \text{DP}(\alpha_j) \\
\alpha_j &\stackrel{\text{iid}}{\sim} \text{Gamma}(0.75, 1).
\end{aligned}$$

where  $\text{Gamma}(a, b)$  denotes a Gamma distribution with expected value equal to  $a/b$ .

- Independent Pitman-Yor Process

$$\begin{aligned}
X_{j,i} \mid (P_1, \dots, P_J) &\stackrel{\text{ind}}{\sim} P_j \quad \text{for } i = 1, 2, \dots \\
P_j \mid \sigma_j, \alpha_j &\stackrel{\text{ind}}{\sim} \text{PYP}(\sigma_j, \alpha_j) \\
\sigma_j &\stackrel{\text{iid}}{\sim} \text{Beta}(1, 3) \quad \alpha_j \stackrel{\text{iid}}{\sim} \text{Gamma}(0.2, 1).
\end{aligned}$$

where Beta denotes a Beta distribution.

- Additive Dirichlet Process

$$\begin{aligned}
X_{j,i} \mid (P_1, \dots, P_J) &\stackrel{\text{ind}}{\sim} P_j \quad \text{for } i = 1, 2, \dots \\
P_j &= \epsilon_j Q_0 + (1 - \epsilon_j) Q_j \\
\epsilon_j &\stackrel{\text{iid}}{\sim} 0.15 \delta_0 + 0.15 \delta_1 + 0.7 \text{Uniform}(0, 1) \\
Q_j \mid \alpha_j &\stackrel{\text{ind}}{\sim} \text{DP}(\alpha_j) \quad \text{for } j = 0, 1, \dots, J \\
\alpha_0 &\stackrel{\text{iid}}{\sim} \text{Gamma}(0.5, 2), \quad \alpha_j \stackrel{\text{iid}}{\sim} \text{Gamma}(6, 2) \quad \text{for } j = 1, 2, \dots, J.
\end{aligned}$$

- Additive Pitman-Yor Process

$$\begin{aligned}
X_{j,i} \mid (P_1, \dots, P_J) &\stackrel{\text{ind}}{\sim} P_j \quad \text{for } i = 1, 2, \dots \\
P_j &= \epsilon_j Q_0 + (1 - \epsilon_j) Q_j \\
\epsilon_j &\stackrel{\text{iid}}{\sim} 0.1 \delta_0 + 0.1 \delta_1 + 0.8 \text{Uniform}(0, 1) \\
Q_j \mid \sigma_j, \alpha_j &\stackrel{\text{ind}}{\sim} \text{PYP}(\sigma_j, \alpha_j) \quad \text{for } j = 0, 1, \dots, J \\
\sigma_0 &\stackrel{\text{iid}}{\sim} \text{Beta}(1, 3), \quad \sigma_j \stackrel{\text{iid}}{\sim} \text{Beta}(1, 2) \quad \text{for } j = 1, 2, \dots, J \\
\alpha_0 &\stackrel{\text{iid}}{\sim} \text{Gamma}(0.25, 4), \quad \alpha_j \stackrel{\text{iid}}{\sim} \text{Gamma}(2, 2) \quad \text{for } j = 1, 2, \dots, J.
\end{aligned}$$

- Hierarchical Dirichlet Process

$$\begin{aligned}
X_{j,i} \mid (P_1, \dots, P_J) &\stackrel{\text{ind}}{\sim} P_j \quad \text{for } i = 1, 2, \dots \\
P_j \mid Q &\stackrel{\text{iid}}{\sim} \text{DP}(\alpha, Q), \\
Q &\sim \text{DP}(\alpha_0, P_0) \\
\alpha_0 &\stackrel{\text{iid}}{\sim} \text{Gamma}(1, 1/3), \quad \alpha_j \stackrel{\text{iid}}{\sim} \text{Gamma}(1, 1/2) \quad \text{for } j = 1, 2, \dots, J.
\end{aligned}$$

- Hierarchical Pitman-Yor Process

$$\begin{aligned}
X_{j,i} \mid (P_1, \dots, P_J) &\stackrel{\text{iid}}{\sim} P_j \quad \text{for } i = 1, 2, \dots \\
P_j \mid Q &\stackrel{\text{iid}}{\sim} \text{PYP}(\sigma, \alpha, Q), \\
Q &\sim \text{PYP}(\sigma_0, \alpha_0, P_0) \\
\sigma_0 &\stackrel{\text{iid}}{\sim} \text{Beta}(1, 2), \quad \sigma_j \stackrel{\text{iid}}{\sim} \text{Beta}(1, 2) \quad \text{for } j = 1, 2, \dots, J \\
\alpha_0 &\stackrel{\text{iid}}{\sim} \text{Gamma}(1, 1), \quad \alpha_j \stackrel{\text{iid}}{\sim} \text{Gamma}(1, 1) \quad \text{for } j = 1, 2, \dots, J.
\end{aligned}$$

The choice of the parameters of the hyperpriors on discount and concentration parameters is performed as follows. We use the values suggested in Battiston *et al.* (2018) for the Hierarchical Pitman-Yor Process, and then we fix the ones of the other strategies considering the probabilities of ties as a function of the hyperparameters and approximately match their expected values and variances. This selection procedure ensures a fair performance comparison, as the probabilities of ties provide an excellent summary of dependence for rmSSPs. The resulting expected probability of ties and corresponding variances are reported in Table S.1.

| Model           | $\mathbb{E}[\text{prob tie across}]$ | $\mathbb{V}[\text{prob tie across}]$ | $\mathbb{E}[\text{prob tie within}]$ | $\mathbb{V}[\text{prob tie within}]$ |
|-----------------|--------------------------------------|--------------------------------------|--------------------------------------|--------------------------------------|
| Independent DP  | 0                                    | 0                                    | 0.672                                | 0.049                                |
| Independent PYP | 0                                    | 0                                    | 0.669                                | 0.047                                |
| +DP             | 0.388                                | 0.092                                | 0.666                                | 0.052                                |
| +PY             | 0.400                                | 0.064                                | 0.628                                | 0.038                                |
| HDP             | 0.389                                | 0.056                                | 0.671                                | 0.041                                |
| HPY             | 0.397                                | 0.043                                | 0.638                                | 0.033                                |

Table S.1: Expected probabilities of ties within and across as functions of the hyperparameters and corresponding variances. Values are obtained via Monte Carlo approximation simulating 2000 samples of the hyperparameters from the hyperpriors per each model.

To sample the concentration parameters of the Dirichlet processes, we employed a Gibbs Sampler via an augmented representation of the full-conditional of the concentration parameter, avoiding a Metropolis within the Gibbs step. For the hyperparameters of the Pitman-Yor processes, we devised an adaptive Metropolis-Hasting, obtained via 10 repeated steps within the main Gibbs algorithm. At each of the 30 sequential sampling steps of the multi-armed bandit problem, we perform 200 iterations of the MCMC algorithm, leading to a total of 6000 iterations (not including the Metropolis-Hasting steps, when present) per strategy. After observing a new data point in a sequential step, we initialize the MCMC for the next step with a warm start based on the last iteration of the MCMC output in the previous step. For instance, we initialize the values of the hyperparameters with the last sampled value in the previous MCMC chain that targets their posterior distribution without conditioning to the new data point.

Moreover, for hierarchical processes, we perform 1000 iterations of the MCMC before estimating the probability of discovery at the first sequential sampling step to achieve a

warm start also at the first sampling step. Code for all six strategies is freely available at <https://github.com/GiovanniRebaudo/MSSP>.

## References

- Antoniak, C. E. (1974). Mixtures of Dirichlet processes with applications to Bayesian non-parametric problems. *Ann. Stat.*, **2**, 1152–1174.
- Battiston, M., Favaro, S., and Teh, Y. W. (2018). Multi-armed bandit for species discovery: a Bayesian nonparametric approach. *J. Am. Stat. Assoc.*, **113**, 455–466.
- Blackwell, D. and MacQueen, J. B. (1973). Ferguson distributions via Pólya urn schemes. *Ann. Stat.*, **1**, 353–355.
- De Blasi, P., Favaro, S., Lijoi, A., Mena, R. H., Prünster, I., and Ruggiero, M. (2015). Are Gibbs-type priors the most natural generalization of the Dirichlet process? *IEEE Trans. Pattern Anal. Mach. Intell.*, **37**, 212–229.
- Ferguson, T. S. (1973). A Bayesian analysis of some nonparametric problems. *Ann. Stat.*, **1**, 209–230.
- Ghosal, S. and van der Vaart, A. (2017). *Fundamentals of Nonparametric Bayesian Inference*. Cambridge Univ. Press.
- Gnedin, A. V. and Pitman, J. (2006). Exchangeable Gibbs partitions and Stirling triangles. *J. Math. Sci.*, **138**, 5674–5685.
- Green, P. J. and Richardson, S. (2001). Modelling heterogeneity with and without the Dirichlet process. *Scand. J. Stat.*, **28**, 355–375.
- Lee, J., Quintana, F. A., Müller, P., and Trippa, L. (2013). Defining predictive probability functions for species sampling models. *Stat. Sci.*, **28**, 209–222.
- Lijoi, A., Mena, R. H., and Prünster, I. (2005). Hierarchical mixture modeling with normalized inverse-Gaussian priors. *J. Am. Stat. Assoc.*, **100**, 1278–1291.
- Lijoi, A., Mena, R. H., and Prünster, I. (2007). Controlling the reinforcement in Bayesian non-parametric mixture models. *J. R. Stat. Soc. Series B Stat. Methodol.*, **69**, 715–740.
- Miller, J. W. and Harrison, M. T. (2018). Mixture models with a prior on the number of components. *J. Am. Stat. Assoc.*, **113**, 340–356.
- Nobile, A. (1994). *Bayesian Analysis of Finite Mixture Distributions*. Ph.D. thesis, Carnegie Mellon Univ.
- Nobile, A. and Fearnside, A. T. (2007). Bayesian finite mixtures with an unknown number of components: the allocation sampler. *Stat. Comput.*, **17**, 147–162.

- Pitman, J. (1996). Some developments of the Blackwell-MacQueen urn scheme. *Lect. Notes-Monogr. Series*, **30**, 245–267.
- Pitman, J. (2006). *Combinatorial Stochastic Processes*. Springer.
- Pitman, J. and Yor, M. (1997). The two-parameter Poisson-Dirichlet distribution derived from a stable subordinator. *Ann. Probab.*, **25**, 855–900.
- Richardson, S. and Green, P. J. (1997). On Bayesian analysis of mixtures with an unknown number of components (with discussion). *J. R. Stat. Soc. Series B Stat. Methodol.*, **59**, 731–792.
